# Supplementary material for: The Cost of Privacy: Rates of Convergence for Parameter Estimation with Differential Privacy
Source: arXiv:1902.04495 source file (2026-09-18)
Supplement: Supplementary file 1 [file Supplement.tex]

\documentclass[letterpaper,12pt]{article}
\usepackage{amsmath,amssymb,amsthm,graphicx,xcolor,mathrsfs}
\usepackage{setspace}
\usepackage{bbm, bm}
\usepackage{url}
\usepackage[colorlinks,linkcolor=black, citecolor=blue,urlcolor=blue]{hyperref}
\usepackage[numbers]{natbib}
\usepackage{varwidth}
\usepackage[ruled, linesnumbered, lined, commentsnumbered, resetcount,algosection]{algorithm2e}
\usepackage{multirow}
\usepackage{xr}
%\externaldocument{Main}
\usepackage{cancel}
\usepackage[normalem]{ulem}
\usepackage{subfig, float}
\usepackage{rotating}
\usepackage{array}
\allowdisplaybreaks

\newcommand{\PreserveBackslash}[1]{\let\temp=\\#1\let\\=\temp}
\newcolumntype{C}[1]{>{\PreserveBackslash\centering}p{#1}}

\usepackage[latin1]{inputenc}

\numberwithin{equation}{section}
\theoremstyle{plain}

\numberwithin{Theorem}{section}

\numberwithin{Lemma}{section}
{
	\theoremstyle{definition}

	\numberwithin{example}{section}
	
	\numberwithin{fact}{section}

}

\addtolength{\textwidth}{1in} \addtolength{\oddsidemargin}{-0.5in}
\addtolength{\textheight}{1.2in} \addtolength{\topmargin}{-0.62in}

\begin{document}
	
\title{Supplement to ``The Cost of Privacy: Optimal Rates of Convergence for Parameter Estimation with Differential Privacy''\footnote{The research was supported in part by NSF grant DMS-1712735 and NIH grants R01-GM129781 and R01-GM123056.}}
\author{T. Tony Cai, \; Yichen Wang, \; and \; Linjun Zhang\\
	University of Pennsylvania}
\maketitle
\begin{abstract}
	This document includes the proofs omitted in the main text of ``The Cost of Privacy: Optimal Rates of Convergence for Parameter Estimation with Differential Privacy''. Section \ref{sec: ub proofs} contains proofs of upper bound results (Theorems \ref{thm: low-dim mean upper bound}, \ref{thm: high-dim mean upper bound}, \ref{thm: low-dim regression upper bound} and \ref{thm: high-dim regression upper bound}) and their related auxiliary lemmas. Section \ref{sec: lb proofs} contains proofs of lower bound results (Theorems \ref{thm: low-dim mean lower bound}, \ref{thm: high-dim mean lower bound}, \ref{thm: low-dim regression lower bound} and \ref{thm: high-dim regression lower bound}) and their related auxiliary lemmas. 
\end{abstract}

\newpage
\tableofcontents

\newpage
\appendix 
\include{A_Proofs_upper_bound}
\include{B_Proofs_lower_bound}

%%%%%%%%%%%%%%%%%%%%%%%%%%%%%%%%%%%%%%%%%%%%%%%%%%%%%%%%%%%%%%%%
\bibliographystyle{plain}
\bibliography{reference}

\end{document}
